# Supplementary material for: DiNAT-IR: Exploring Dilated Neighborhood Attention for High-Quality Image Restoration
Source: arXiv:2507.17892 source file (2026-11-05)
Supplement: Supplementary file 1 [file appendix.tex]

\section{Appendix}
\subsection{Training Configurations}

\noindent
{\bftab GoPro:} We train DiNAT-IR with an image patch size of $256 \times 256$ and a batch size of 16 for 600K iterations with PSNR loss. The initial learning rate is set as $3 \times 10^{-4}$, gradually decreasing to $1 \times 10^{-6}$ following the cosine annealing learning scheme. AdamW is used as the optimizer, and the betas is set to $[0.9, 0.999]$. We further fine tune DiNAT-IR with an image size of $384 \times 384$ and a batch size of 8 for another 200K iterations, inspired by the progressive training strategy introduced in Restormer~\citep{zamir2022restormer} and Stripformer~\citep{tsai2022stripformer}. The initial learning rate is set as $1 \times 10^{-4}$. We observe that DiNAT-IR may not fully converge to the optimal point, which implies that an improved training strategy may boost model performance on the GoPro dataset~\citep{nah2017deep}. The network at the last iteration is selected as our motion deblurring model.

\noindent
{\bftab DPDD:} We train DiNAT-IR with an image size of $256 \times 256$ and a batch size of 16 for 300K iterations with PSNR loss. The optimizer and learning scheduler settings are similar to the motion deblurring task. We select the model at the 290K iteration as our dual-focus defocus deblurring network. As to the single-image defocus deblurring task, we use the model at the 140K iteration as the final version.

\noindent
{\bftab Rain13k:} We train DiNAT-IR with an image size of $256 \times 256$ and a batch size of 16 for 300K iterations with L1 loss. The optimizer and learning scheduler settings are similar to the motion deblurring task. We further fine tune DiNAT-IR with an image size of $384 \times 384$ and a batch size of 8 for another 100K iterations, and the network at the 40K iteration is chosen as our deraining model.

\noindent
{\bftab SIDD:} We train DiNAT-IR with an image size of $256 \times 256$ and a batch size of 16 for 300K iterations with PSNR loss. The optimizer and learning scheduler settings are similar to the motion deblurring task. The network at the 220K iteration is chosen as our denoising model.
